# Supplementary material for: Peristaltic elastic instability in an inflated cylindrical channel
Source: arXiv:1805.02998 ancillary file (2018-05-08)
Supplement: Supplementary file 1 [file Theoretical_SI.pdf]

# Peristaltic elastic instability in an inflated cylindrical channel: Theoretical Supplement

N. Cheewaruangroj & J. S. Biggins

Here we provide full algebraic details of our stability analysis of an inflated cylindrical channel. As in our main manuscript, we consider neo-Hookean body initially occupying $a < r < b$, and subject to an inflationary interior fluid pressure $P_{in}$ which causes it to undergo a displacement field $\mathbf{u}$. If $F = I + \nabla\mathbf{u}$ ($F_{ij} = \delta_{ij} + \partial_j u_i$) is the deformation gradient and $\sigma = \frac{\partial W}{\partial F} = \left(\mu F - P\mathrm{Det}\left(F\right)F^{-T}\right)$, is the PK1 large deformation stress, then we show in the main manuscript that the deformation will be governed by the bulk equations

$$\nabla\cdot\sigma = 0 \implies \mu\nabla^2\mathbf{u} - \mathrm{Det}\left(F\right)F^{-T}\cdot\nabla P = 0 \tag{1}$$

$$\mathrm{Det}(F) = 1, \tag{2}$$

and the boundary conditions

$$\left(\sigma + P_f\mathrm{Det}\left(F\right)F^{-T}\right)\cdot\hat{\mathbf{r}}\Big|_{r=a,b} = 0. \tag{3}$$

We restrict attention to axisymmetric displacements $\mathbf{u} = (u_r, 0, u_z)$. Since we are working in cylindrical coordinates, we first recall the forms of the gradient operators in the above equations, using commas to denote partial derivatives:

$$\nabla P = \begin{pmatrix} P_{,r} \\ 0 \\ P_{,z} \end{pmatrix} \qquad \nabla\mathbf{u} = \begin{pmatrix} u_{r,r} & 0 & u_{r,z} \\ 0 & \frac{u_r}{r} & 0 \\ u_{z,r} & 0 & u_{z,z} \end{pmatrix} \qquad \nabla^2\mathbf{u} = \begin{pmatrix} u_{r,rr} + \frac{u_{r,r}}{r} - \frac{u_r}{r^2} + u_{r,zz} \\ 0 \\ u_{z,rr} + \frac{u_{z,r}}{r} + u_{z,zz} \end{pmatrix}. \tag{4}$$

Before considering the peristaltic instability we first consider the systems uniform dilation:

$$\mathbf{u} = u_0(r)\hat{\mathbf{r}} \qquad P = \mu P_0(r). \tag{5}$$

The terms become

$$\nabla P = \mu\begin{pmatrix} P_0' \\ 0 \\ 0 \end{pmatrix} \qquad \nabla^2\mathbf{u} = \begin{pmatrix} u_0'' + \frac{u_0'}{r} - \frac{u_0}{r^2} \\ 0 \\ 0 \end{pmatrix}. \tag{6}$$

and the deformation gradient $F$ and $\mathrm{Det}\left(F\right)F^{-T}$ are then

$$F = \begin{pmatrix} 1+u_0' & 0 & 0 \\ 0 & 1+\frac{u_0}{r} & 0 \\ 0 & 0 & 1 \end{pmatrix}, \quad \mathrm{Det}\left(F\right)F^{-T} = \begin{pmatrix} 1+\frac{u_0}{r} & 0 & 0 \\ 0 & 1+u_0' & 0 \\ 0 & 0 & 1+u_0'+\frac{u_0}{r}(1+u_0') \end{pmatrix} \tag{7}$$

Using these expressions, eqn. (1) & (2) become

$$r^2u_0'' + ru_0' - u_0 - r\left(r+u_0\right)P_0' = 0, \qquad u_0 + \left(r+u_0\right)u_0' = 0, \tag{8}$$

which are solved by

$$u_0(r) = \sqrt{r^2+c^2} - r \equiv R - r, \qquad P_0(r) = \frac{1}{2}\left(\frac{r^2}{r^2+c^2} - \ln\left(\frac{r^2}{r^2+c^2}\right)\right) + q, \tag{9}$$

where $c$ and $q$ are constants that are determined by the boundary conditions (3) at $r = a$ and $r = b$,

$$\left(\frac{P_{in}}{\mu} - P_0(a)\right)(a + u_0(a)) + a(1 + u_0'(a)) = 0, \tag{10}$$

$$-P_0(b)(b + u_0(b)) + b(1 + u_0'(b)) = 0. \tag{11}$$

By substituting (9) into (10,11) , we obtain expression for $q$ and $P_{in}$ as a function of $c$

$$q = \frac{1}{2}\left[\frac{b^2}{b^2+c^2} + \ln\left(\frac{b^2}{b^2+c^2}\right)\right], \tag{12}$$

$$\begin{aligned} P_{in} &= \frac{\mu}{2}\left[\ln\left(\frac{b^2}{b^2+c^2}\right) - \ln\left(\frac{a^2}{a^2+c^2}\right) + \frac{b^2}{b^2+c^2} - \frac{a^2}{a^2+c^2}\right] \\ &= \frac{\mu}{2}\left[-\ln\left(1+(a/b)^2(\lambda^2-1)\right) + \ln\left(\lambda^2\right) + \frac{1}{1+(a/b)^2(\lambda^2-1)} + \frac{1}{\lambda^2}\right] \\ &= \frac{\mu}{2}\left[g(1+(a/b)^2(\lambda^2-1)) - g(\lambda^2)\right], \end{aligned} \tag{13}$$

where $\lambda = \sqrt{a^2+c^2}/a$ and function $g(x) \equiv (1/x) - \ln(x)$. In the limit of $b \to \infty$, eqn (13) becomes

$$P_{in} = \frac{\mu}{2}\left[1 + \ln(\lambda^2) - \lambda^{-2}\right]. \tag{14}$$

We then apply the small perturbation $\mathbf{u} = u_0(r)\hat{\mathbf{r}} + \delta\mathbf{u}$ and $P = \mu P_0(r) + \delta P$. They induce the first order change in the deformation gradient $\delta F = \nabla\delta\mathbf{u}$ and the PK1 stress

$$\begin{aligned} \delta\sigma &= \mu\delta F - \delta\left(P\mathrm{Det}\left(F\right)F^{-T}\right) \\ &= \mu\delta F - \delta P F_0^{-T} - \mu P_0\delta\left(\mathrm{Det}\left(F\right)F^{-T}\right), \end{aligned} \tag{15}$$

where $F_0$ is the unperturbed deformation gradient. We also use the fact that $\mathrm{Det}\left(F_0\right) = 1$ to simplify the expression. Equations (1) and (2) need to be satisfied by the perturbation:

$$\nabla\cdot\delta\sigma = 0 \implies \mu\nabla^2\delta\mathbf{u} - F_0^{-T}\cdot\nabla\delta P - \mu\delta\left(\mathrm{Det}\left(F\right)F^{-T}\right)\cdot\nabla P_0 = 0 \tag{16}$$

$$\delta\mathrm{Det}(F) = 0 \implies \mathrm{Tr}\left(F_0^{-1}\delta F\right) = 0. \tag{17}$$

with the perturbed boundary conditions

$$\left[\delta\sigma - P_f\delta\left(\mathrm{Det}\left(F\right)F^{-T}\right)\right]\cdot\hat{\mathbf{r}}\Big|_{r=a,b} = 0. \tag{18}$$

Using an sinusoidal perturbation as an anzats:

$$\delta\mathbf{u} = f_r(r)\cos(kz)\hat{\mathbf{r}} + f_z(r)\sin(kz)\hat{\mathbf{z}}, \qquad \delta P = \mu P_1(r)\cos(kz). \tag{19}$$

We then have

$$\nabla\delta P = \mu\begin{pmatrix} P_1'\cos(kz) \\ 0 \\ -kP_1\sin(kz)\end{pmatrix}, \qquad \nabla^2\delta\mathbf{u} = \begin{pmatrix}\left(f_r'' - k^2 f_r + \frac{f_r'}{r} - \frac{f_r}{r^2}\right)\cos(kz) \\ 0 \\ \left(f_z'' - k^2 f_z + \frac{f_z'}{r}\right)\sin(kz)\end{pmatrix}, \tag{20}$$

$$\delta F = \begin{pmatrix} f_r'\cos(kz) & 0 & -kf_r\sin(kz) \\ 0 & -\frac{f_r}{r}\cos(kz) & 0 \\ f_z'\sin(kz) & 0 & kf_z\cos(kz)\end{pmatrix}, \tag{21}$$

$$\delta\left(\mathrm{Det}\left(F\right)F^{-T}\right) = \begin{pmatrix}\frac{f_r + kRf_z}{r}\cos(kz) & 0 & -\frac{R}{r}f_z'\sin kz \\ 0 & (f_r' + \frac{kr}{R}f_z)\cos(kz) & 0 \\ \frac{kR}{r}f_r\sin(kz) & 0 & (\frac{f_r}{R} + \frac{R}{r}f_r')\cos kz\end{pmatrix}. \tag{22}$$

Only the terms at first order in the perturbation are included. The bulk equations (16,17), after some simplifications, are then

$$rR^4\left(rf_r'' + f_r' - RP_1'\right) + r^2 f_r\left(r^2 - R^2\left(k^2R^2+2\right)\right) + kRf_z\left(r^2 - R^2\right)^2 = 0, \tag{23}$$

$$kf_r\left(r^2 - R^2\right)^2 + rR^3\left(rf_z'' + f_z' - k^2 rf_z + krP_1\right) = 0, \tag{24}$$

$$R\left(Rf_r' + krf_z\right) + rf_r = 0. \tag{25}$$

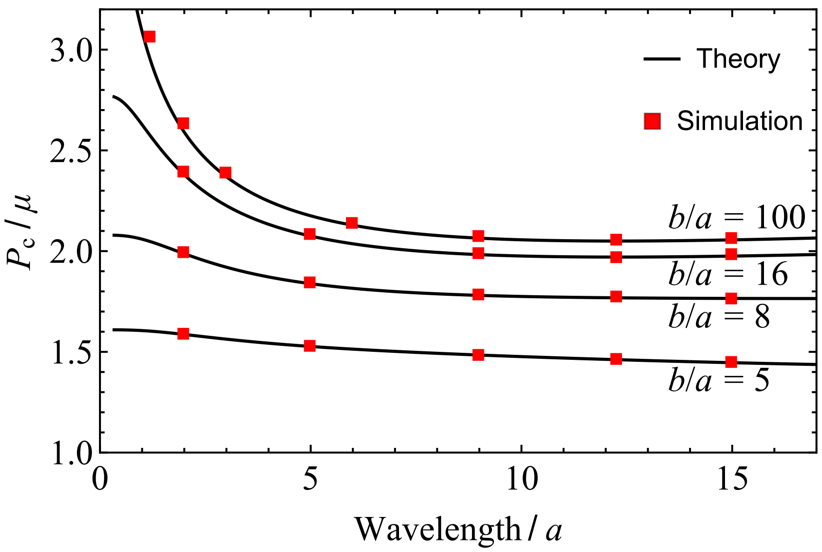


FIG. 1. numerical results and theoretical prediction for threshold cavity pressure at different radii ratio $b/a$ as a function of wavelength. For $b/a > 100$, the curve would be on top of the $b/a = 100$ curve, showing the convergence

Equation (24) and (25) and provide expressions for $f_z$ and $P_1$:

$$f_z(r) = -\frac{rf_r(r) + R^2 f_r'(r)}{krR}, \tag{26}$$

$$P_1(r) = \frac{rR^3(k^2 r f_z(r) - f_z'(r) - r f_z''(r)) - k(R^2 - r^2)^2 f_r(r)}{kr^2R^3}. \tag{27}$$

Substituting these expressions into (23), we obtain a forth order differential equation for $f_r$:

$$R^2 \Bigg[ f_r' \left(-2k^2r^4 - r^2\left(1 - k^2R^2\right) - 3R^2\right) + r \Big[ f_r'' \left(-k^2r^4 + r^2\left(1 - k^2R^2\right) + 3R^2\right)$$

$$+ r\left(rR^2 f_r^{(4)} + f_r^{(3)}\left(r^2 - 2R^2\right)\right)\Big]\Bigg] + k^2 r f_r \left(r^4\left(k^2R^2 - 2\right) + r^2R^2 + 2R^4\right) = 0. \tag{28}$$

The boundary conditions (18) at $r = a$ and $r = b$ are

$$R(a)f_z'(a) - kaf_r(a) = 0 \tag{29}$$

$$aR(a)^2 f_r'(a) - a^2 f_r(a) - ka^2R(a)f_z(a) - R(a)^3P_1(a) = 0 \tag{30}$$

$$R(b)f_z'(b) - kbf_r(b) = 0 \tag{31}$$

$$bR(b)^2 f_r'(b) - b^2 f_r(b) - kb^2R(b)f_z(b) - R(b)^3P_1(b) = 0, \tag{32}$$

where $R(x) = \sqrt{x^2 + c^2}$. The differential equation is complicated and not easy to solve analytically. Instead, we solve it using Matlab's bvp4c boundary value solver. We specify values for $a, b$ and $k$ then bvp4c is able to find the lowest value for $c$ for which the equations have a solution, and find the solution. We then iterate over $k$ to find the solution with lowest $c$. The threshold cavity pressure can then be calculated from $c$ via eqn (13). This would be the critical value of $P_{in}$ for the instability and its wavenumber. In Fig. 1, we plot the threshold value of $P_{in}$ against wavelength, $2\pi/k$, at different values of $b/a$, showing the convergence as $b/a \to \infty$. We also performed numerical simulation which agrees with our prediction. For $b \to \infty$, the minimum is at $P_{in} = 2.052\mu$ and $2\pi/k = 12.278a$ as stated in the main text.
