# Supplementary material for: Peristaltic elastic instability in an inflated cylindrical channel
Source: arXiv:1805.02998 ancillary file (2018-05-08)
Supplement: Supplementary file 2 [file experiment_SI.pdf]

# Peristaltic elastic instability in inflated cylindrical channel: Experimental Supplement

Nontawit Cheewaruangroj and John S. Biggins
*Cavendish Laboratory, University of Cambridge, 19 JJ Thomson Avenue, Cambridge CB3 0HE, United Kingdom*

Karolis Leonavicius and Shankar Srinivas
*Department of Physiology Anatomy and Genetics, University of Oxford, Oxford OX1 3QX, UK*
(Dated: May 8, 2018)

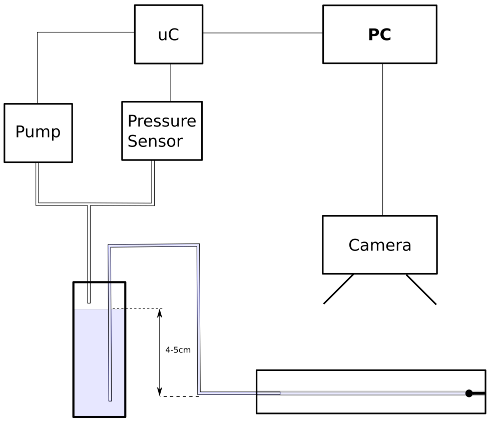


FIG. 1. Schematic experimental setup

Hydrogel channels of different modulus were made by moulding different concentrations of polyacrylamide/bisacrylamide mixture (39:1) in 1mm thick slabs around 30$\mu$m wires. The wires were 35mm in length and cast inside a hydrogel slab whose length was 12mm. The mixture was then polymerized into a solid gel using a mixture of ammonium persulfate (0.1%) and tetra ethyl methyl diamine (TEMED, 1%) and the wire was pulled out to leave a cylindrical channel. Finally, phosphate buffered saline (PBS) was used to equilibrate the gels for 30 minutes after polymerization, prior to the experiments. Such cavities were made in batches of 5.

The channel inflation was achieved using the experimental setup shown in fig. 1. To pressurize the channels, a computer controlled diaphragm air pump was connected to a glass capillary containing PBS solution. One of the capillary ends was pulled under flame to a 100–300$\mu$m diameter in order to fit into the channel inside the hydrogel. A glass bead was used to plug the other side of the hydrogel channel. The pressure in the channel was then increased in stages of approximately 200Pa, each lasting at least 2s until the elastic deformation occurred. The resulting channel deformations were then imaged using a CMOS camera sensor fitted to a Leica stereomicroscope eyepiece. The images were processed manually using ImageJ software to measure the diameter of the channel at each recorded pressure value as well as the peristaltic wavelength in channels beyond the threshold of instability.

Five different hydrogel compositions were used, ranging between 4–5% bisacrylamide, to provide a range of shear moduli. The shear modulus, $\mu$ was measured by comparing the relationship between the channel dilation $\lambda$ and the cavity pressure while the channel is stable,

$$P_{in} = \frac{\mu}{2}\left[1 + \log(\lambda^2) - \lambda^{-2}\right].$$

As seen in Fig. 2, the measured modulii agree well with the literature values [1] for a given composition, validating the accuracy and equilibrium of the mechanical measurements.

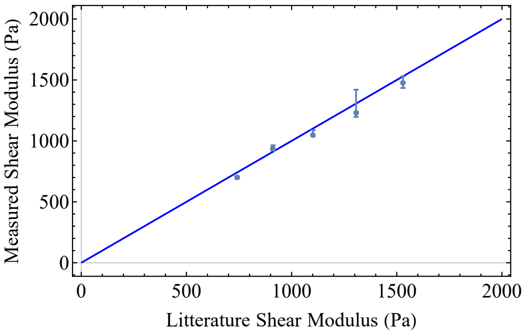


FIG. 2. Measured hydrogel modulus vs value expected from composition. Each point combines multiple pressure-dilation measurements from five independent hydrogel channels.

The threshold pressure was measured as the lowest pressure required for the peaks to appear in the channel profile. For each gel composition, this critical pressure was measured in five different cavities. These five results were averaged to produce the threshold figure 2b in the main text. In each cavity, the wavelength was also measured for each pressure beyond threshold to give the experimental wavelength points in fig 2c in the main text.

After unloading a channel, and waiting for at most $\sim$10 minutes for the gel to fully relax, it was found the instability measurement experiments could be repeated in exactly the same manner.

To generate the cell-growth driven instability in Fig. 5 in the main paper, mouse embryonic stem cells were cultured in T-25 flasks coated with 0.1% w/v gelatin until passage number 50-60. The cell culture media consisted of 90% DMEM medium (Gibco), 10% fetal calf serum

(FCIII, Hyclone), 1mM sodium pyruvate, 1mM non-essential amino acid mix, 0.1mM $\beta$-mercaptoethanol, 2mM L-glutamine and 103U/mL leukaemia inducible factor (LIF). During this stage, cells were passaged every 2 days and seeded at 400,000 cells per T25 flask. A dense cell suspension was then injected (with a micropipette) into a 40 micrometer diameter channel through a 5% polyacrylamide gel, manufactured as described above. The cell culture grew within the channel for ten days, while the cell culture media was exchanged every other day, Tissue growth caused the channel to expand, and the peristaltic instabilities started to appear after 7 days of culture.

[1] J. R. Tse and A. J. Engler, Current protocols in cell biology , 10 (2010).
